# Supplementary material for: Trust the Ray, Not the Depth: Ray-Lateral Agreement for Multi-View 3D Human Pose Fusion
Source: arXiv:2611.23513 source file (2026-11-17)
Supplement: Supplementary file 1 [file supp_labels.tex]

% Numbers of the supplementary material's sections, figures and tables cited in the main text;
% the supplement is not part of this version.
\makeatletter
\newlabel{fig:camera_count}{{6}{3}{\textbf {Error against camera count} on Panoptic: median (left) and 95th percentile (right, log scale) of MPJPE over camera subsets. All pairs; \pinfo {3}{subsets} random subsets with three and four cameras, \pinfo {5}{subsets} at each larger count marked, up to 25; and all 31 cameras together. We plot the 95th percentile because the maximum depends on how many subsets we sample. \method and the hybrid use held-out parameters}{figure.caption.35}{}}
\newlabel{fig:camera_count@cref}{{[figure][6][]6}{[1][2][]3}{}{}{}}
\newlabel{fig:supp_cameras}{{8}{4}{The 31 HD cameras of \texttt {171204\_pose1} seen from above, numbered as in the dataset; each triangle points along the camera's optical axis and is coloured by its height above the floor. Grey: the reference pelvis positions of the six people}{figure.caption.39}{}}
\newlabel{fig:supp_cameras@cref}{{[figure][8][]8}{[1][2][]4}{}{}{}}
\newlabel{fig:supp_failures}{{10}{6}{\textbf {Failures of \method } on Panoptic, chosen by rule as in \cref {fig:qualitative}: (g) its largest error over all pairs; (h) the pair and frame where its error exceeds that of DLT the most; (i) its largest error over all three-camera subsets}{figure.caption.43}{}}
\newlabel{fig:supp_failures@cref}{{[figure][10][]10}{[1][4][]6}{}{}{}}
\newlabel{fig:supp_qualitative}{{9}{5}{\textbf {More cases on Panoptic}, chosen by rule as in \cref {fig:qualitative}: (d) the largest error of DLT over all pairs; (e) that of RANSAC over all three-camera subsets; (f) a typical case, the median frame of the three-camera subset with the median error of \method }{figure.caption.42}{}}
\newlabel{fig:supp_qualitative@cref}{{[figure][9][]9}{[1][4][]5}{}{}{}}
\newlabel{fig:supp_subjects}{{7}{3}{The six people of Panoptic \texttt {171204\_pose1}, one frame each from camera 00\_05, with faces blurred}{figure.caption.37}{}}
\newlabel{fig:supp_subjects@cref}{{[figure][7][]7}{[1][2][]3}{}{}{}}
\newlabel{sec:exp_runtime}{{6.8}{6}{\texorpdfstring {\hskip -1em.~}{}Runtime}{subsection.6.8}{}}
\newlabel{sec:exp_runtime@cref}{{[subsection][8][6]6.8}{[1][6][]6}{}{}{}}
\newlabel{sec:supp_baselines}{{6.4}{1}{\texorpdfstring {\hskip -1em.~}{}Baselines}{subsection.6.4}{}}
\newlabel{sec:supp_baselines@cref}{{[subsection][4][6]6.4}{[1][1][]1}{}{}{}}
\newlabel{sec:supp_fit3d}{{6.10}{7}{\texorpdfstring {\hskip -1em.~}{}A second dataset: Fit3D}{subsection.6.10}{}}
\newlabel{sec:supp_fit3d@cref}{{[subsection][10][6]6.10}{[1][7][]7}{}{}{}}
\newlabel{sec:supp_hmr2}{{6.7}{4}{\texorpdfstring {\hskip -1em.~}{}Other per-view estimators}{subsection.6.7}{}}
\newlabel{sec:supp_hmr2@cref}{{[subsection][7][6]6.7}{[1][4][]4}{}{}{}}
\newlabel{sec:supp_mle}{{6.2}{1}{\texorpdfstring {\hskip -1em.~}{}Fusion as maximum likelihood}{subsection.6.2}{}}
\newlabel{sec:supp_mle@cref}{{[subsection][2][6]6.2}{[1][1][]1}{}{}{}}
\newlabel{sec:supp_panoptic}{{6.5}{2}{\texorpdfstring {\hskip -1em.~}{}Panoptic details}{subsection.6.5}{}}
\newlabel{sec:supp_panoptic@cref}{{[subsection][5][6]6.5}{[1][2][]2}{}{}{}}
\newlabel{sec:supp_qualitative}{{6.6}{2}{\texorpdfstring {\hskip -1em.~}{}Qualitative results}{subsection.6.6}{}}
\newlabel{sec:supp_qualitative@cref}{{[subsection][6][6]6.6}{[1][2][]2}{}{}{}}
\newlabel{sec:supp_seq2}{{6.9}{7}{\texorpdfstring {\hskip -1em.~}{}A second Panoptic sequence}{subsection.6.9}{}}
\newlabel{sec:supp_seq2@cref}{{[subsection][9][6]6.9}{[1][6][]7}{}{}{}}
\newlabel{sec:supp_shift}{{6.3}{1}{\texorpdfstring {\hskip -1em.~}{}Translating rather than rescaling the depth}{subsection.6.3}{}}
\newlabel{sec:supp_shift@cref}{{[subsection][3][6]6.3}{[1][1][]1}{}{}{}}
\newlabel{tab:ablation}{{2}{2}{\textbf {Ablation} on Panoptic: median over the \gnum {ab}{3@subsets} three-camera subsets of \cref {tab:panoptic} and the \gnum {ab}{5@subsets} five-camera subsets of \cref {fig:camera_count} (mm). Each fusion variant has its own parameters chosen by leave-one-subject-out from the grid used for \method . Bold: lowest per column}{table.caption.28}{}}
\newlabel{tab:ablation@cref}{{[table][2][]2}{[1][1][]2}{}{}{}}
\newlabel{tab:depth}{{4}{3}{\textbf {Depth correction} on Panoptic: median over the 31 single cameras and the \gnum {dc}{pairs} camera pairs; 507 frames, six subjects weighted equally (mm). Without correction, averaging misplaces the body by about a metre. Rescaling every depth compresses the body along the ray; translating along the ray (\cref {eq:shift}) keeps its shape. True $\mK _c$: SAM~3D~Body receives each camera's true intrinsics and needs no correction. Triangulation does not use the corrected depth. \method with the held-out parameters of \cref {tab:panoptic}}{table.caption.36}{}}
\newlabel{tab:depth@cref}{{[table][4][]4}{[1][2][]3}{}{}{}}
\newlabel{tab:hmr2}{{8}{7}{\textbf {Other per-view estimators} on the camera subsets of \cref {tab:panoptic}: median and worst MPJPE over subsets (mm). CameraHMR with its own focal-length estimate, corrected by \cref {eq:shift}. RANSAC at the 20\,px of \cref {tab:panoptic}, and with its threshold $\tau $ chosen by leave-one-subject-out (three or more cameras); hybrid: RANSAC set (20\,px) + \method ; held-out parameters. PA-MPJPE and all baselines: \cref {tab:supp_hmr2,tab:supp_camerahmr_fov}. Bold: best per column and estimator}{table.caption.44}{}}
\newlabel{tab:hmr2@cref}{{[table][8][]8}{[1][5][]7}{}{}{}}
\newlabel{tab:supp_bones}{{5}{3}{Median reference bone lengths per identity of \texttt {171204\_pose1}. They differ by up to \gnum {bl}{spread}\%, consistent with six different people rather than re-tracks of one}{table.caption.38}{}}
\newlabel{tab:supp_bones@cref}{{[table][5][]5}{[1][2][]3}{}{}{}}
\newlabel{tab:supp_camerahmr}{{11}{9}{\textbf {CameraHMR given each camera's true focal length}: the camera subsets, frames and methods of \cref {tab:panoptic} (mm). Held-out: $(\lambda ,\alpha )$ chosen by leave-one-subject-out. Bold: best in each column}{table.caption.50}{}}
\newlabel{tab:supp_camerahmr@cref}{{[table][11][]11}{[1][6][]9}{}{}{}}
\newlabel{tab:supp_camerahmr_fov}{{10}{8}{\textbf {CameraHMR as the per-view estimator}, with its own focal-length estimate (HumanFoV) corrected by \cref {eq:shift}: the camera subsets, frames and methods of \cref {tab:panoptic} (mm). Held-out: $(\lambda ,\alpha )$ chosen by leave-one-subject-out. Bold: best in each column}{table.caption.49}{}}
\newlabel{tab:supp_camerahmr_fov@cref}{{[table][10][]10}{[1][6][]8}{}{}{}}
\newlabel{tab:supp_detector}{{3}{3}{\textbf {The 2D detector pipeline} on the camera subsets of \cref {tab:panoptic}: YOLOv8x-pose keypoints triangulated four ways, scored on the joints each method produces (coverage: the share of the $507\times 17$ joints with a result, mean over subsets); the SAM~3D~Body rows are from \cref {tab:panoptic}, with held-out parameters, and cover every joint. Median and worst over subsets, six subjects weighted equally (mm). Bold: best in each column}{table.caption.33}{}}
\newlabel{tab:supp_detector@cref}{{[table][3][]3}{[1][2][]3}{}{}{}}
\newlabel{tab:supp_hmr2}{{9}{8}{\textbf {HMR~2.0 as the per-view estimator}: the camera subsets, frames and methods of \cref {tab:panoptic} (mm). Held-out: $(\lambda ,\alpha )$ chosen by leave-one-subject-out. Bold: best in each column}{table.caption.48}{}}
\newlabel{tab:supp_hmr2@cref}{{[table][9][]9}{[1][6][]8}{}{}{}}
\newlabel{tab:supp_joints}{{7}{4}{\textbf {Per joint} on Panoptic: median MPJPE over the \gnum {sj}{subsets} four-camera subsets of \cref {tab:panoptic}, left and right joints averaged, subjects weighted equally (mm). Parameters as in \cref {tab:supp_subjects}. Bold: lowest per joint}{table.caption.41}{}}
\newlabel{tab:supp_joints@cref}{{[table][7][]7}{[1][2][]4}{}{}{}}
\newlabel{tab:supp_seq2}{{12}{9}{\textbf {A second Panoptic sequence} (\texttt {\gnum {p2}{name}}, \gnum {p2}{subjects} subjects weighted equally, \gnum {p2}{scored} frames): every pair, and random subsets of three and four of the 31 HD cameras (mm). The setting of $(\lambda ,\alpha )$ per camera count is the one selected on the first sequence; nothing is tuned here. Bold: best in each column}{table.caption.51}{}}
\newlabel{tab:supp_seq2@cref}{{[table][12][]12}{[1][6][]9}{}{}{}}
\newlabel{tab:supp_subjects}{{6}{4}{\textbf {Per subject} on Panoptic: for each subject, the median MPJPE over the subsets of \cref {tab:panoptic} (mm). \method and the hybrid use the setting chosen on the other five subjects; All: the median of the six-subject mean, as in \cref {tab:panoptic}. With two cameras, DLT+IRLS and RANSAC reduce to DLT. Bold: lowest per subject and camera count}{table.caption.40}{}}
\newlabel{tab:supp_subjects@cref}{{[table][6][]6}{[1][2][]4}{}{}{}}
\makeatother
